# Supplementary material for: Spotlight the Negatives: A Generalized Discriminative Latent Model
Source: arXiv:1507.02144 source file (2015-07-08)
Supplement: Supplementary file 1 [file SupMat.pdf]

# Supplementary Material

## 1 Intuitive example of LVM and GLVM

Figure 1 gives intuitive examples of positive and negative latent variables.

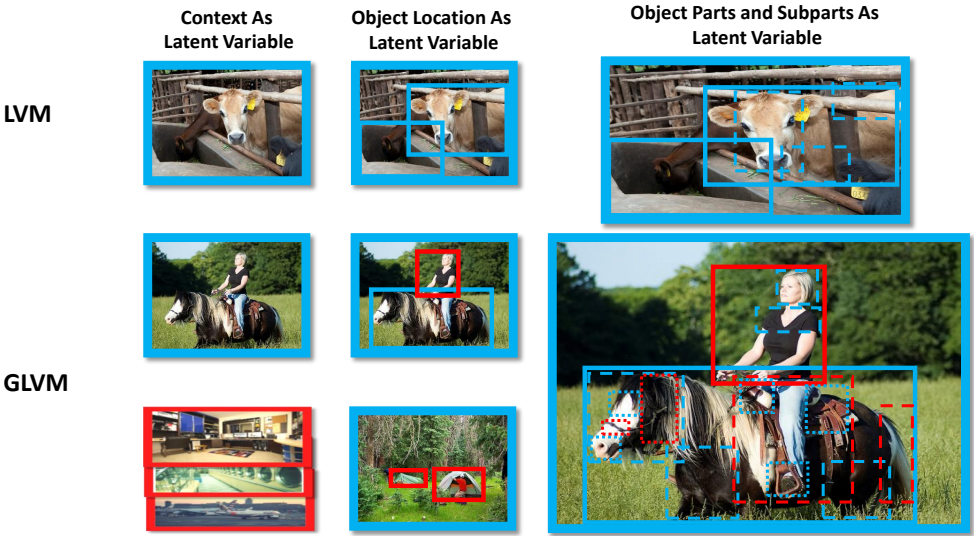

Figure 1: **Intuitive example of LVM and GLVM.** Assume the task of *cow* image classification. This figure visualizes examples of possible latent variables for LVM and GLVM models. A latent variable can be assigned at image level such as the background scene and then gradually go down a hierarchy of objects, parts and subparts. Positive latent variables (modeling evidences for cow) of an LVM may correspond to different scenes where cow is likely to be seen *e.g.* stable, meadow (blue boxes in the first column). Another positive latent variable can be assigned to the location of the cow in the image (second column, first row). In addition, location of different parts of cow *e.g.* head, back, legs can be modeled as other latent variables dependent to the latent variable of cow location (top right). All these examples of latent variables in LVMs look for evidences for the existence of cow. In GLVM we encourage the modeling of counter evidences through negative latent variables. For example at high level a negative latent variable may correspond to scenes where cow is unlikely to be found *e.g.* office, laundromat, or airport (bottom left). Meadow is an evidence for cow, but cows are less likely to be seen in a meadow beside camping tents (a dependent negative latent variable to positive latent variable meadow). Horses are visually similar to cow but people usually do not ride cows thus a human on top of cow can be negative evidence (a negative latent variable dependent to the positive latent variable of cow location). Furthermore, human, a negative latent variable for cow, can have its own positive latent variable as parts *e.g.* face and shoulders (bottom right).

## 2 Dependency Structure

Complexity of evaluating GLVM scoring function is governed by the dependency structure of the underlying feature function  $\phi$ . In the most extreme case, with no independence assumption at all, evaluating the scoring function would require exhaustive search on the space of all possible assignments of the latent variables. This grows exponentially with the number of latent variables and becomes intractable very quickly.

Tree-structured dependencies are particularly interesting and widely used in practice [10, 11]. Complexity of evaluating the scoring function with tree-structured dependency is quadratic in the cardinality of the domain of a single latent variable.

Dependency structure of the feature function also affects the complexity of finding the fixed latent assignments in inference functions of training, and hence, the construction of the bounds  $B_t$ .

Another note is that although we call  $a_k$ s positive latent variables and  $b_k$ s negative latent variables, this is only for simplicity of notation and explanations. That is, the true meaning of these variables as evidences or counter evidences for the positive class changes by the dependency structure of the scoring function. For example a negative latent variable depending on another negative latent variable of the positive class is not a counter evidence for positive class nor is a evidence. Conversely, positive latent variables dependent to a negative latent variable act as a counter evidence for the positive class.

## 3 Algorithm

Details of the training framework is given in Section 4 of the main paper. Here is the algorithm corresponding to the training procedure of GLVM. The equation numbers refer to the main paper.

---

**Algorithm 1** Training GLVM classifiers.      Note that equation numbers refer to the main paper.

---

**Input:**  $D = \{(x_i, y_i)\}_{i=1}^n, w_0$

$t \leftarrow 0$

**repeat**

    Construct  $\tilde{S}_t(w)$  from Equation (11) and  $w_t$

    Construct  $\hat{S}_t(w)$  from Equation (12) and  $w_t$

    Construct  $B_t(w)$  from Equation (8)

$w_{t+1} \leftarrow \arg \min_w B_t(w)$

$t \leftarrow t + 1$

**until**  $w_t$  does not change

**Output:**  $w_t$

---

## 4 Deformable Part Models

Part based models have had a long and successful presence in the history of Computer Vision [12, 13, 14, 15, 16].

Deformable Part Models (DPMs) [17] have been extensively used for object detection over the past decade. Despite their incredible flexibility to object deformation and viewpoint changes they only look for positive evidence in images. In particular, DPMs do not capture

counter evidence. For example, the knowledge that a cow-head detector fires strongly on a detection window should decrease the score of horse-detector on that window. We propose an extension to DPMs by augmenting them with negative parts. We call our model *Generalized-DPM* (or GDPM in short).

Training of the proposed model does not fit in the latent SVM framework [9]. We propose an algorithm to learn DPMs with negative parts. Our experimental results show that negative parts complement DPMs [9]. DPM is a mixture of multi-scale part-based object detectors. Each mixture component captures appearance of the object in a specific viewpoint. Each mixture has a *root* filter for capturing the global structure of the object in a coarse scale. It also has a set of *deformable part* filters for capturing parts of the object individually in a higher resolution. DPM uses sliding window search to detect objects. The root filter is used as the detection window during training. Consider a DPM with  $n$  parts. We denote the location (and size) of the root filter and the parts by  $r$  and  $l = (l_1, \dots, l_n)$  respectively. We also denote the choice of the mixture component by  $c$ . The true root, and part locations as well as the choice of the mixture component are unknown even during training and, therefore, are treated as latent variables in a DPM.

We define a *latent configuration* as an assignment of all latent variables in the model and denote it by  $z = (c, r, l)$ . Score of a DPM with latent configuration  $z$  on image  $x$  is a linear function of the model parameters, which we denote by  $\beta$ , and is defined as follows:

$$g_\beta(x, z) = \beta \cdot \Phi(x, z) \quad (1)$$

where  $\Phi(x, z)$  extracts features from image  $x$  according to the latent configuration  $z$ .

Let  $R$  be a set of candidate root locations (for examples, all detection windows that have high overlap with a given image region). We denote the detection score on  $R$  by  $f_\beta(x, R)$  and define it as the score of the best latent configuration that places the root filter at a location in  $R$  as follows:

$$f_\beta(x, R) = \max_{\substack{z=(r,c,l) \\ s.t. \ r \in R}} g_\beta(x, z) \quad (2)$$

## 4.1 Training Deformable Part Models

Let  $\mathcal{D} = \{(x_i, y_i, b_i)\}_{i=1}^N$  denote a set of  $N$  annotated training examples.  $x_i$  denotes an image.  $y_i \in \{+1, -1\}$  denotes a class label that determines whether the example is foreground ( $y_i = +1$ ) or background ( $y_i = -1$ ).  $b_i$  denotes the coordinates of the annotated bounding box that circumscribes the object in a foreground image.  $b_i$  is irrelevant if  $y_i = -1$ . All root filter locations on a background image are considered as independent negative examples.

DPM uses the root filter as a detection window during training. Despite availability of  $b_i$ 's for foreground images, DPM treats true detection bounding boxes on the foreground images as latent variables. Any root filter whose overlap with the annotated bounding box  $b_i$  exceeds a certain threshold  $\tau$  is considered as a valid detection (true positive) for  $b_i$ . We denote the set of valid detections of  $b_i$  by  $H(x_i, b_i, \tau)$ . In order to train DPMs a separate training set  $D = \{(x_i, y_i, R_i)\}_{i=1}^N$  is constructed from the annotated examples in  $\mathcal{D}$ . Each background example  $(x, y = -1, b_i) \in \mathcal{D}$  adds multiple examples  $(x, y, \{r\})$  to  $D$ , one for each root placement  $r$ . Each foreground example  $(x, y = +1, b_i) \in \mathcal{D}$  adds one example  $(x, y, R)$  to  $D$  where  $R = H(x, b, \tau)$ . In DPM, the value of  $\tau$  is set to 0.7.

DPM uses Latent SVM [9] for training. Given the training set  $D$ , the model parameters  $\beta$  are trained by minimizing the following objective function:

$$O(\beta) = \frac{1}{2} \|\beta\|^2 + C \sum_{i=1}^N \max\{0, 1 - y_i f_\beta(x_i, R_i)\} \quad (3)$$

The objective function in Equation 3 is non-convex. Particularly,  $f_\beta(x_i, R_i)$  as defined in Equation 2 is maximum of a set of linear functions  $g_\beta(x, z)$ , and therefore is convex. Then for samples with  $y > 0$  the hinge loss in Equation 3 becomes concave.

Latent SVM employs an alternating approach similar to CCCP [9] to minimize the training objective. CCCP is an iterative procedure that alternates between 1) constructing a convex upper bound on the original objective function and 2) optimizing the bound. CCCP is guaranteed to converge to a local minimum of the original objective function.

In the case of DPMs, the first step boils down to fixing the value of the latent variables in Equation 3 for *foreground* examples. Let  $z_i = (r_i, c_i, l_{i,1}, \dots, l_{i,n})$  denote a particular assignment of the latent variables for the foreground example  $(x_i, y_i, R_i)$ . A convex upper bound to  $O(\beta)$  is defined as follows:

$$\begin{aligned} B(\beta) = & \frac{1}{2} \|\beta\|^2 + C \sum_{\substack{i=1 \\ y_i=-1}}^N \max\{0, 1 + f_\beta(x_i, R_i)\} \\ & + C \sum_{\substack{i=1 \\ y_i=+1}}^N \max\{0, 1 - g_\beta(x_i, z_i)\} \end{aligned} \quad (4)$$

We call this the *relabeling* step of the training algorithm.

The second step involves solving the following optimization problem:

$$\beta^* = \arg \min_{\beta} B(\beta) \quad (5)$$

Any assignment of  $z_i$ 's for foreground examples leads to a convex function (Equation 4) which is an upper bound to  $O$  (Equation 3). In order to guarantee progress in each iteration we require that  $z_i$ 's are set to the maximum scoring configurations under the previous model  $\beta^*$  as follows:

$$z_i = \arg \max_z g_{\beta^*}(x_i, z), \forall i \text{ s.t. } y_i = +1 \quad (6)$$

## 4.2 Negative Parts

In a binary classifier, a negative (positive) part is defined as a part whose *maximum* response is *subtracted* from (*added* to) the classification score [9].

While positive parts collect evidence for presence of an object negative parts collect *counter-evidence* for it. For example, consider a detection window  $\omega$ . Presence of a *saddle* in the detection window  $\omega$  should decrease the score of a *cow* detector on  $\omega$ . This is because *cows* tend not to have *saddles* on their backs. Thus, if we find a *saddle* in the detection window of a *cow* detector we, most likely, are confusing a *horse* for a *cow*. Counter evidence is particularly important in discriminating between similar objects; like *cow* from *horse* in

the hypothetical example above. We obtain this behavior by augmenting *cow* detector model with a negative part that fires on *saddle*.

Finally, we note that standard DPMs cannot capture counter-evidence. For example, if  $F$  is the appearance model of a positive part,  $-F$  does *not* make it a negative part. In this paper we extend DPMs by augmenting them with negative parts.

### 4.3 Adding Negative Parts to Deformable Part Models

In DPM, responses of all part filters are *added* to the detection score of the classifier. Thus, DPMs cannot model negative parts. We generalize DPMs by augmenting them with negative parts. We call the proposed model *Generalized-DPM* (or GDPM in short). Standard DPM [9] is a GDPM with zero negative parts.

We denote a GDPM with  $k$  mixture components by  $\gamma = (\gamma_1; \dots; \gamma_k)$ . Each mixture component captures the appearance of the object in a viewpoint. A mixture component with  $n$  positive parts and  $m$  negative parts is parameterized by  $\gamma_c = (F_{c,0}; w_{c,1}^+; \dots; w_{c,n}^+; w_{c,1}^-; \dots; w_{c,m}^-)$ .  $F_{c,0}$  denotes the root filter,  $w_j^+$ 's denote the positive part models, and  $w_j^-$ 's denote the negative part models. Each part model  $w_{c,j} = (F_{c,j}; d_{c,j})$  has an appearance  $F_{c,j}$  and a deformation parameter vector  $d_{c,j}$ .

Let  $l^+ = (l_1^+, \dots, l_n^+)$  denote the positive part placements and  $l^- = (l_1^-, \dots, l_m^-)$  denote the negative part placements. We denote a latent configuration in a GDPM by  $z = (r, c, l^+, l^-)$ . Score of a GDPM  $\gamma$  with latent configuration  $z$  on image  $x$  is a linear function of the model parameters  $\gamma$ . We denote this by  $g_\gamma(x, z)$  and define it as follows:

$$g_\gamma(x, z) = \gamma \cdot \Phi(x, z) \quad (7)$$

where  $\Phi$  extracts features from image  $x$  according to the latent configuration  $z$ . This is very similar to the score function of the standard DPM (see Equation 1). For example, both functions are linear in the model parameters. Detection score of placing the root at  $r$ , however, is fundamentally different for the two models. For example, unlike Equation 2 we *cannot* compute  $f_\gamma(x, R)$  by maximizing over all the latent variables. We will elaborate more on the differences between  $f_\beta(x, R)$  and  $f_\gamma(x, R)$  in the rest of this section.

Like in DPM, part dependencies in GDPM respect a star configuration with the root filter at the center of the star. Thus, part placements are independent given the location of the root filter. Let  $\phi_a(x, l_j)$  denote appearance features extracted from patch  $l_j$  of image  $x$  (e.g. HOG features). Also let  $\phi_d(l_j, r)$  denote the deformation features of placing part  $j$  at  $l_j$  given that the root filter is placed at  $r$ . We define the feature function  $\phi(x, l_j, r) = (\phi_a(x, l_j); \phi_d(l_j, r))$ . For DPMs, we can rewrite Equation 2 as follows:

$$\begin{aligned} f_\beta(x, R) = \max_{r \in R} \max_{c=1}^k & F_{c,0} \cdot \phi_a(x, r) \\ & + \sum_{j=1}^n \max_{l_j} w_{c,j} \cdot \phi(x, l_j, r) \end{aligned} \quad (8)$$

In contrast, for GDPMs we have:

$$\begin{aligned}
 f_{\gamma}(x, R) = & \max_{r \in R} \max_{c=1}^k F_{c,0} \cdot \phi(x, r) \\
 & + \sum_{j=1}^n \max_{l_j^+} w_{c,j}^+ \cdot \phi(x, l_j^+, r) \\
 & - \sum_{j=1}^m \max_{l_j^-} w_{c,j}^- \cdot \phi(x, l_j^-, r)
 \end{aligned} \tag{9}$$

One way to see that GDPM is more general than DPM is to note that the score function of Equation 8 is convex in the model parameters whereas Equation 9 is not.

#### 4.4 Training with Negative Parts

We define the training objective of a GDPM as follows:

$$O(\gamma) = \frac{1}{2} \|\gamma\|^2 + C \sum_{i=1}^N \max\{0, 1 - y_i f_{\gamma}(x_i, R_i)\} \tag{10}$$

This objective function is non-convex. Moreover, unlike DPMs, fixing the latent variables for the foreground examples does *not* make it convex. Thus, we cannot use Latent SVM framework to train GDPMs.

We deploy CCCP for training the objective function of Equation 10. Recall that CCCP alternates between constructing a convex function that upper bounds the original objective function and optimizing the bound.

We obtain a convex upper bound  $B(\gamma)$  to the training objective by replacing  $f_{\gamma}(x_i, R_i)$  with a convex upper bound  $\check{f}_{\gamma}$  for background images and a concave lower bound  $\hat{f}_{\gamma}$  for foreground images.

$$\begin{aligned}
 B(\gamma) = & \frac{1}{2} \|\gamma\|^2 + C \sum_{\substack{i=1 \\ y_i=-1}}^N \max\{0, 1 + \check{f}_{\gamma}(x_i, R_i)\} \\
 & + C \sum_{\substack{i=1 \\ y_i=+1}}^N \max\{0, 1 - \hat{f}_{\gamma}(x_i, R_i)\}
 \end{aligned} \tag{11}$$

In the rest of this section we first explain how the bounds are constructed and then elaborate on the optimization of the bound.

#### 4.5 Constructing Convex Bounds

In this section we explain how we obtain  $\check{f}_{\gamma}$  and  $\hat{f}_{\gamma}$  in order to construct the bound  $B(\gamma)$  in Equation 11. Let  $\gamma^*$  be the solution to the previous convex bound. We define  $l_{i,j}^-(r, c) = \arg \max_l w_{c,j}^- \cdot \phi(x_i, l, r)$  to be the optimal placement of the  $j$ -th negative part using the previous model conditioned on the choice of the root location  $r$  and the mixture component  $c$ .

We obtain  $\check{f}_\gamma$  by fixing the placement of the negative parts according to  $l_{i,j}^-(r, c)$  as follows:

$$\begin{aligned} \check{f}_\gamma(x_i, R_i) = & \max_{r \in R} \max_{c=1}^k F_{c,0} \cdot \phi(x_i, r) \\ & + \sum_{j=1}^n \max_{l_j^+} w_{c,j}^+ \cdot \phi(x_i, l_j^+, r) \\ & - \sum_{j=1}^m w_{c,j}^- \cdot \phi(x_i, l_{i,j}^-(r, c), r) \end{aligned} \quad (12)$$

Let  $(r_i, c_i, l_i^+)$  denote the best placement of the root filter, choice of the mixture component, and placement of the positive parts using the model  $\gamma^*$  given that the negative parts have been placed optimally according to  $l_{i,j}^-(r, c)$ . We can formally define this as follows:

$$\begin{aligned} (r_i, c_i, l_i^+) = & \arg \max_{(r, c, l)} F_{c,0}^* \cdot \phi(x_i, r) \\ & + \sum_{j=1}^n w_{c,j}^{*+} \cdot \phi(x_i, l_j, r) \\ & - \sum_{j=1}^m w_{c,j}^{*-} \cdot \phi(x_i, l_{i,j}^-(r, c), r) \end{aligned} \quad (13)$$

We obtain  $\hat{f}_\gamma$  as follows:

$$\begin{aligned} \hat{f}_\gamma(x_i, R_i) = & F_{c_i,0} \cdot \phi(x_i, r_i) \\ & + \sum_{j=1}^n w_{c_i,j}^+ \cdot \phi(x_i, l_{i,j}^+, r_i) \\ & - \sum_{j=1}^m \max_{l_j^-} w_{c_i,j}^- \cdot \phi(x_i, l_j^-, r_i) \end{aligned} \quad (14)$$

## 4.6 Initializing Negative Parts

The positive parts in original DPM [1] is initialized by first learning a root filter (whole object detector without parts). Then in order to initialize the location and weights of a part filter, a submatrix of root filter is sought which has the maximal positive energy. Positive energy is measured by sum of squared *positive* weights in the submatrix of the root filter. The first part is initialized with the best submatrix location and weights. Then all the weights are zeroed at that location and the procedure is repeated to initialize a second part. This continues until the desired number of parts are added. We initialize positive parts in the same manner. Also, we initialize the negative part similarly, except that we try to find the submatrix with highest negative energy being sum of squared *negative* weights of the submatrix. This involves the main results of the paper.

We further initialize the negative parts with the positive parts of similar classes. Particularly, we initialize the negative parts for *cow* GDPM model by taking positive parts from *horse* DPM model.

## 4.7 Inference for Data Mining

When doing inference for GDPM data mining, we need to construct a concave lower bound for positive samples and convex upper bound for negative samples. That is, we need to fix the position of negative parts for negative samples at the location of relabeling. We further need to fix the location of positive parts, mixture component and root filter location for positive samples to the assignments at the relabeling. On the other hand, the positive parts and mixture component needs to be maximized for negative samples and negative parts needs to be updated for positive samples. Storing the fixed values of latent variables for all negative samples (hundreds of thousands negative bounding box for each image) is prohibitively memory-consuming. Thus, in our implementation, we do the following. At each relabeling step we keep a copy of the model. We also store the inferred component and location of the root filter only for positive samples (requires low amount of memory since number of positive annotations are usually low). Then at each iteration of data mining: For positive samples we take the current model and roll back the positive parts to the copied model, and do the inference at the saved location and with the saved component. As for negative examples, we take the current model and roll back the negative parts to the copied model and do the inference. This way we simply take care of convex upper bound and concave lower bounds with low memory footprint. However, this comes at the cost of two times more computational complexity. Since the main complexity of the inferences goes back to convolution of part/root filters, the remedy for this would be to save the output of convolution for positive parts on positive examples and negative parts on negative examples (proportional to the number of images and independent of number of negative bounding boxes per image).



# 5 Dataset

Random images from Cat Head dataset [1]. Note that, many of the cat heads are not frontal.

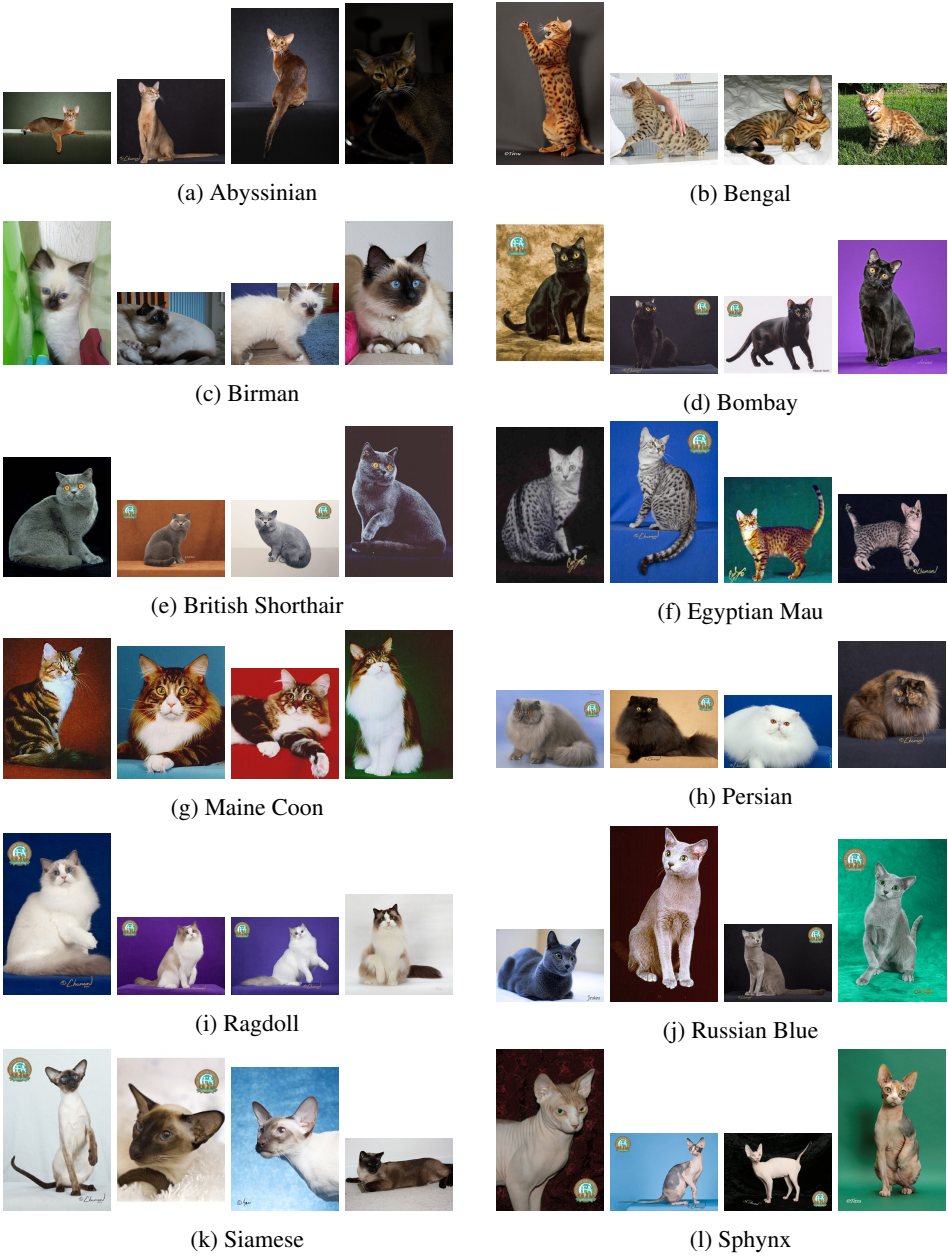

Figure 2: Samples of Pet [1] dataset used for cat head detection

## 6 Precision Recall Curves

In this section, the precision recall curves for DPM comparing with its best performing GDPM variant is plotted for animals subset of PASCAL VOC 2007. For the class of *cow* an extra curve is plotted which belongs to a different initialization of negative parts using *horse* DPM model. For the class of *bird* and *dog* while the AP (calculated by average of 11 sampled points) is equal for GDPM and DPM, the GDPM curve shows slightly better precision at lower recalls.

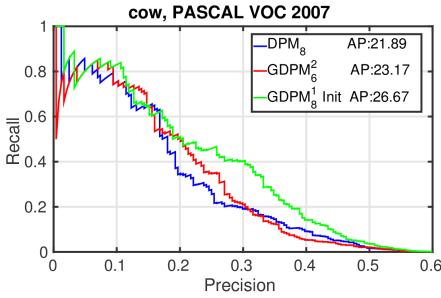

(a) PR curve for *cow* in PASCAL VOC 2007 using original DPM, GDPM with 2 negative parts, and GDPM with one negative part initialized by horse DPM model.

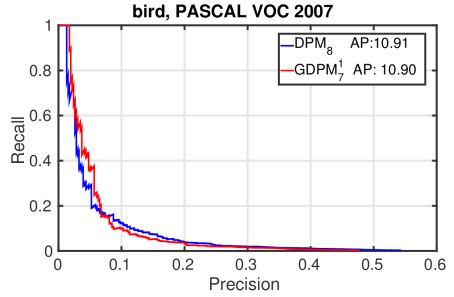

(b) PR curve for *bird* in PASCAL VOC 2007 using original DPM, GDPM with 1 negative part. Although the AP (computed by taking average of 10 sampled points from the curve) is equal, the GDPM curve has slightly higher precision at lower recall.

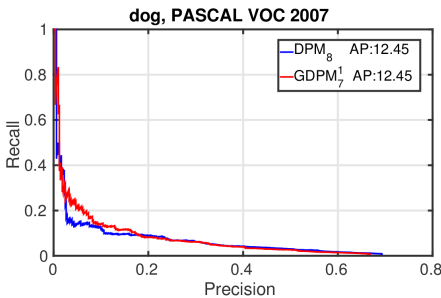

(c) PR curve for *dog* in PASCAL VOC 2007 using original DPM, GDPM with 1 negative part. Although the AP (computed by taking average of 10 sampled points from the curve) is equal, the GDPM curve has slightly higher precision at lower recall.

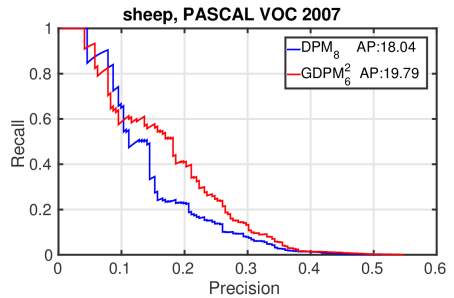

(d) PR curve for *sheep* in PASCAL VOC 2007 using original DPM, GDPM with 2 negative part. The GDPM curve exhibits higher precision at different recalls.

Figure 3: PR curves for animals subset of PASCAL VOC 2007

## References

- [1] Hossein Azizpour and Ivan Laptev. Object detection using strongly-supervised deformable part models. In *ECCV*, 2012.
- [2] Lubomir D. Bourdev and Jitendra Malik. Poselets: Body part detectors trained using 3d human pose annotations. In *ICCV*, pages 1365–1372, 2009.
- [3] Timothy F. Cootes, Gareth J. Edwards, and Christopher J. Taylor. Comparing active shape models with active appearance models. In *BMVC*, pages 1–10, 1999.
- [4] Pedro F. Felzenszwalb, David A. McAllester, and Deva Ramanan. A discriminatively trained, multiscale, deformable part model. In *CVPR*, 2008.
- [5] Bastian Leibe, Ales Leonardis, and Bernt Schiele. Robust object detection with interleaved categorization and segmentation. *IJCV*, 77(1-3):259–289, 2008.
- [6] Sobhan Naderi Parizi, Andrea Vedaldi, Andrew Zisserman, and Pedro F. Felzenszwalb. Automatic discovery and optimization of parts for image classification. In *ICLR*, 2015.
- [7] O. M. Parkhi, A. Vedaldi, A. Zisserman, and C. V. Jawahar. Cats and dogs. In *IEEE Conference on Computer Vision and Pattern Recognition*, 2012.
- [8] Alan Yuille and Anand Rangarajan. The concave-convex procedure. *Neural Computation*, 15(4):915–936, 2003.
- [9] Long Zhu, Yuanhao Chen, and Alan L. Yuille. Learning a hierarchical deformable template for rapid deformable object parsing. *PAMI*, 32(6):1029–1043, 2010.
